# Supplementary material for: A deep learning approach to identify unhealthy advertisements in street view images
Source: arXiv:2007.04611 source file (2021-02-07)
Supplement: Supplementary file 1 [file appendix.tex]

\section{Keywords}

Using a list of keywords that we compiled for \emph{food} (extracting keywords from local food providers and fast-food vendors' menus), \emph{gambling venues}~\footnote{Keywords obtained from Wikipedia: \url{https://en.wikipedia.org/wiki/Category:Gambling_companies_of_the_United_Kingdom}}, \emph{alcohol}~\footnote{Keywords obtained from Wikipedia: \url{https://en.wikipedia.org/wiki/Category:Alcoholic_drink_brands}} and other~\footnote{Our script and keywords can be downloaded from \url{}.}.
